# Supplementary material for: Hyperfine-phonon spin relaxation in a single-electron GaAs quantum dot
Source: arXiv:1711.01474 ancillary file (2017-11-04)
Supplement: Supplementary file 1 [file supplementary.pdf]

## SUPPLEMENTARY MATERIAL

### Hyperfine-phonon spin relaxation in a single-electron GaAs quantum dot

Leon C. Camenzind,<sup>1,\*</sup> Liuqi Yu,<sup>1,\*</sup> Peter Stano,<sup>2,3,4</sup> Jeremy Zimmerman,<sup>5</sup>

Arthur C. Gossard,<sup>5</sup> Daniel Loss,<sup>1,2</sup> and Dominik M. Zumbühl<sup>1</sup>

<sup>1</sup>*Department of Physics, University of Basel, Basel 4056, Switzerland*

<sup>2</sup>*Center for Emergent Matter Science, RIKEN, Saitama 351-0198, Japan*

<sup>3</sup>*Department of Applied Physics, School of Engineering,*

*University of Tokyo, 7-3-1 Hongo, Bunkyo-ku, Tokyo 113-8656, Japan*

<sup>4</sup>*Institute of Physics, Slovak Academy of Sciences, 845 11 Bratislava, Slovakia*

<sup>5</sup>*Materials Department, University of California, Santa Barbara 93106, USA*

## CONTENTS

|                                                                            |    |
|----------------------------------------------------------------------------|----|
| S1. In-plane magnetic field alignment                                      | 2  |
| S2. Level positioning algorithm and sensor stabilization                   | 2  |
| S3. Spin relaxation measurement scheme                                     | 6  |
| S4. Definitions and notations for the electron, nuclear spins, and phonons | 10 |
| S5. The spin relaxation rate                                               | 12 |
| S6. Anisotropy of the hyperfine relaxation rate                            | 14 |
| S7. Dipole matrix elements between the spin opposite states                | 15 |
| S8. Numerical implementation                                               | 17 |
| S9. Parameters and fitting of the spin-orbit constants                     | 17 |
| References                                                                 | 20 |

### S1. IN-PLANE MAGNETIC FIELD ALIGNMENT

For the measurements shown, it is crucial to have a good alignment of the external magnetic field  $\mathbf{B}$  with the plane of the 2DEG. Large enough in-plane magnetic field needs to be applied to induce sufficient Zeeman splitting for energy readout. On the other hand, formation of Landau levels due to the perpendicular magnetic fields must be avoided. We extract the out-of-plane angle  $\xi$  via Hall measurements using the standard van der Pauw geometry. The Hall coefficient  $R_{H,\perp}$  for a perpendicular magnetic field was determined in a separate cool-down. In a parallel field configuration, the finite Hall slope from the out-of-plane field component is  $R_{H,\parallel} = R_{H,\perp} \sin(\xi)$  and depends on the tilt of the device. No quantum oscillations were observed up to 10 T, which indicates that the out-of-plane component of the applied magnetic field is very small. We use a piezo-electric rotator (Fig. 1b) to rotate the device in a 4 T magnetic field. In Fig. S1b,  $\xi$  is plotted as a function of  $\phi$ , the angle with respect to [100] (Fig. S1a). As expected,  $\xi$  shows a sinusoidal behavior in  $\phi$  with periodicity of  $360^\circ$ . We find a maximal misalignment of merely  $1.3^\circ$  close to the crystalline direction [110]. Therefore, we conclude that the effect on our measurements due to the field misalignment is negligible (see Supplementary Section S6).

### S2. LEVEL POSITIONING ALGORITHM AND SENSOR STABILIZATION

The spin relaxation measurement scheme strongly depends on the associated tunneling rates (see Supplementary Section S3) which themselves strongly depend on the energy detuning of ground-state and the chemical potential  $\mu$  of the lead<sup>1</sup>. The dot energy levels drift over time, and to compensate for changes in the tunnel rates, we integrate active stabilization protocols. In this section we first give a brief introduction to resonant tunneling before explaining how

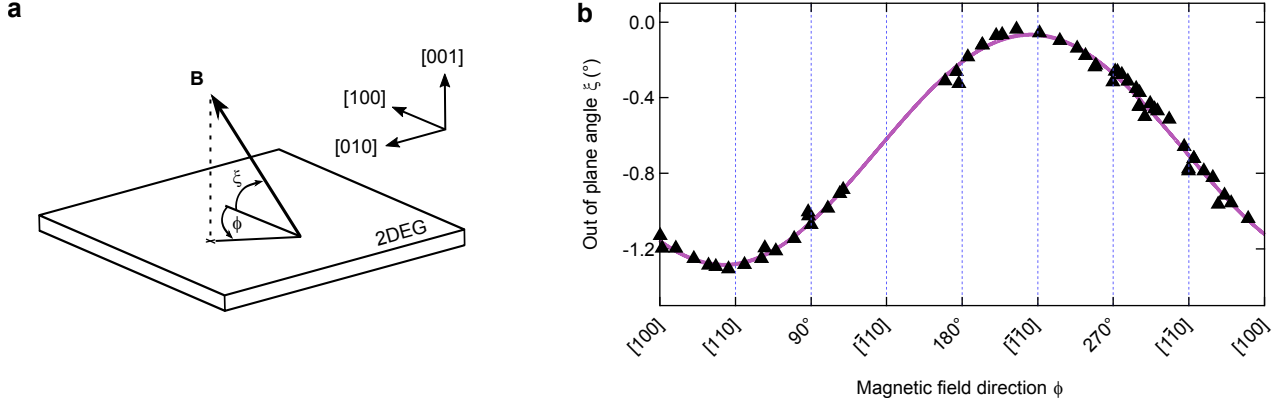

FIG. S1. **In-plane field alignment with 2DEG.** **a** The angles parametrizing the external magnetic field orientation. The small misalignment of the external magnetic field  $B$  with the plane of the 2DEG is described by the out-of-plane angle  $\xi$ . The in-plane angle  $\phi$  is defined as the angle with respect to crystal direction  $[100]$ . **b** The out-of-plane angle  $\xi$  alters as the sample is rotated by the piezoelectric rotator. The data set is very well fitted with a sine of  $2\pi$  periodicity (solid purple curve). Between  $\phi = 115^\circ$  and  $165^\circ$  the sensor of the piezo-rotator does not encode angles.

we exploit this energy dependence for our active level positioning algorithm (LPA)<sup>1</sup>. We then focus on our protocol to maintain the sensitivity of our sensor quantum dot which is also susceptible to fluctuations.

Resonant tunneling of an electron occurs if the occupation probability of the quantum dot is between 0 and 1. In our system, this is observed when the orbital ground-state level of the quantum dot is energetically within the temperature broadening of the 2DEG reservoir (a few  $k_B T$ ) around the lead chemical potential  $\mu$ . An example is presented in Fig. S2a where the dot ground state is aligned with  $\mu$ . Then the occupation probability of the dot is  $1/2$  and electrons resonantly tunnel from the reservoir to the dot and vice versa. The timescale for this tunneling events is given by the details of the tunnel-barrier and is tunable by the surface gates. Quantitatively the tunneling rate at energy  $E$  is  $\Gamma(E) = (2\pi/\hbar)T(E)\rho(E)$  with  $T$  the transmission coefficient and  $\rho$  the density of states in the reservoir<sup>2</sup>. Here, we assume the tunnel-barrier and the corresponding transmission coefficient  $T$  are energy independent for small detuning from  $\mu$  by a few  $k_B T$ .

In Fig. S2b we show an example of resonant tunneling reflected in  $I_{SQD}$ , the current through the sensor quantum dot. We use histograms of  $I_{SQD}$  (Fig. S2c) to distinguish the charge states. For a given waiting time  $t_w$ , we define the total time of the dot being occupied as  $T_{on}$ , and being empty as  $T_{off}$  respectively. The tunnel rate in and out of the quantum dot are then given by  $\Gamma_{in} = N_{total}/(2T_{off})$  and  $\Gamma_{out} = N_{total}/(2T_{on})$  with  $N_{total} = N_{on} + N_{off}$  the total number of tunneling events during  $t_w$ . Another method is to histogram the time intervals where the dot is empty ( $t_{off}$ ) or occupied ( $t_{on}$ ). These times show an exponential distribution (e.g.  $\rho_{off}(t_{off}) \propto \exp(-\Gamma_{in}t_{off})$ ) and the rates can be obtained by fitting. In our experiment, the tunnel rates using these methods are in very good agreement. However, the first method avoids errors induced by binning or fitting, thus is preferred for automatized control. In Fig. S3a-e energy diagrams illustrate  $\mu$ , the ground-state energy of the dot and resonant tunnel rates in ( $\Gamma_{in}$ ) and out ( $\Gamma_{out}$ ) of the dot for five exemplary situations<sup>3,4</sup>. Here the dot level is controlled by adjusting the voltage on the center plunger gate CP (see Fig. 1a in the main text). In Fig. S3a, the ground state is well above  $\mu$  such that an electron on the dot would tunnel out immediately. When the detuning to  $\mu$  is made smaller, occupied

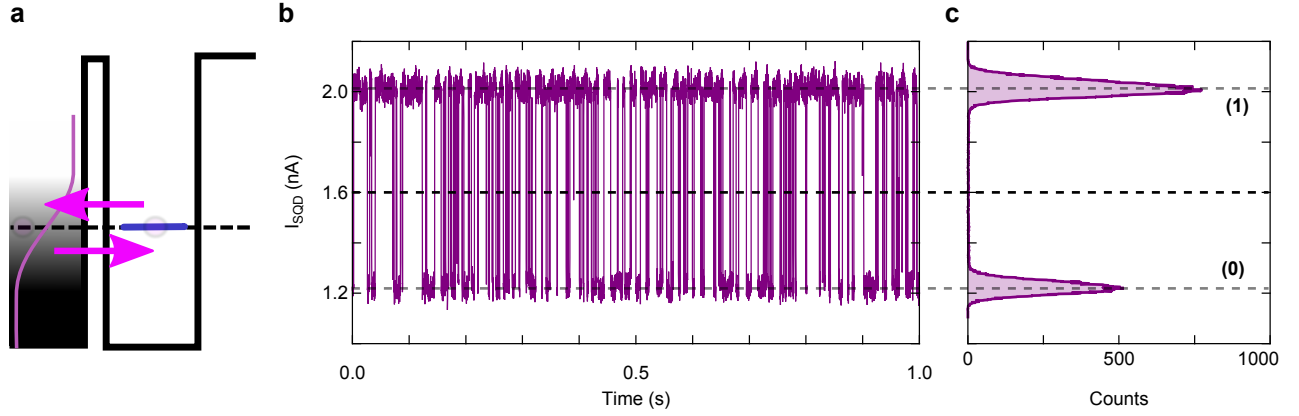

FIG. S2. **Resonant tunneling and discrimination of charge states.** **a** Schematics of resonant tunneling of electrons between the quantum dot and the reservoir. The purple curve indicates the thermal broadening of occupation statistics. This Fermi-Dirac distribution represents the probability of finding an electron in the reservoir as a function of energy. Due to Coulomb blockade we assume no other level is available and the dot is either empty (0) or loaded (1). **b** An exemplary time trace of the resonant tunneling reflected as jumps between two distinguished values of  $I_{SQD}$ . As described in the main text, the tunnel rates  $\Gamma_{on,off}$  are calculated by analyzing such resonant tunneling traces. **c** Histogram of the trace shown in **b** exhibits the two-level system. Due to the large signal-to-noise ratio the charge states (0) and (1) are distinguished with high fidelity. Also, we measure tunnel rates well below the bandwidth of the charge sensor which minimizes errors due to missed events.

states in the reservoir become resonant with the dot level and elastic tunneling could occur (Fig. S3b). Because there are more empty than occupied states in the reservoir, the dot is predominantly empty and  $\Gamma_{off} > \Gamma_{on}$ . When the ground state is aligned with  $\mu$  (Fig. S3c),  $\Gamma_{off} = \Gamma_{on}$  and the dot occupation probability is 1/2. Further lowering the dot level reverses the behavior and  $\Gamma_{off} < \Gamma_{on}$  (Fig. S3d) until there is no available empty state in the reservoir for the electron to elastically tunnel out of the dot (Fig. S3e). In our system we find that inelastic tunneling is strongly suppressed and the electrons are usually trapped for tens of seconds.

Fig. S3f shows the quantitative dependence of  $\Gamma_{in}$  and  $\Gamma_{off}$  on the detuning from  $\mu$ . To illustrate that this behavior is explained by the occupation statistics of the lead, the data is fit to a Fermi-Dirac distribution. The knowledge that the rates are distributed accordingly is used for positioning the ground state relative to  $\mu$  by establishing a closed-loop feedback either on the tunnel rates or on the dot occupation probability.

The feedback protocol is illustrated in Fig. S3f. As shown in the example, the measured tunnel rate off the dot  $\Gamma_{now}$  is feedbacked to adjust the dot level. Therefore a correction  $\Delta E$  is calculated and applied to the plunger gate CP (see in Fig. 1a) to restore the set tunnel rate  $\Gamma_{set}$ . This process is repeated until  $\Gamma_{now}$  is within the tolerance  $\Gamma_{tol}$  around  $\Gamma_{set}$ .

During the spin relaxation measurements, this feedback is performed about every three minutes. As will be discussed in Supplementary Section S3, it is of great significance to have a small, well known and constant  $\Gamma_{off}$  of the spin ground state to guarantee a reliable spin-to-charge conversion. The dot is usually loaded and in Coulomb blockade when the spin excited state becomes resonant such that only resonant tunneling with the spin ground state is visible. In reality, due to the thermal broadening, the spin excited state at the smallest fields also contributes to the total resonant tunneling which distorts the measured rates. However, even if the rates are distorted the tunnel off rates of

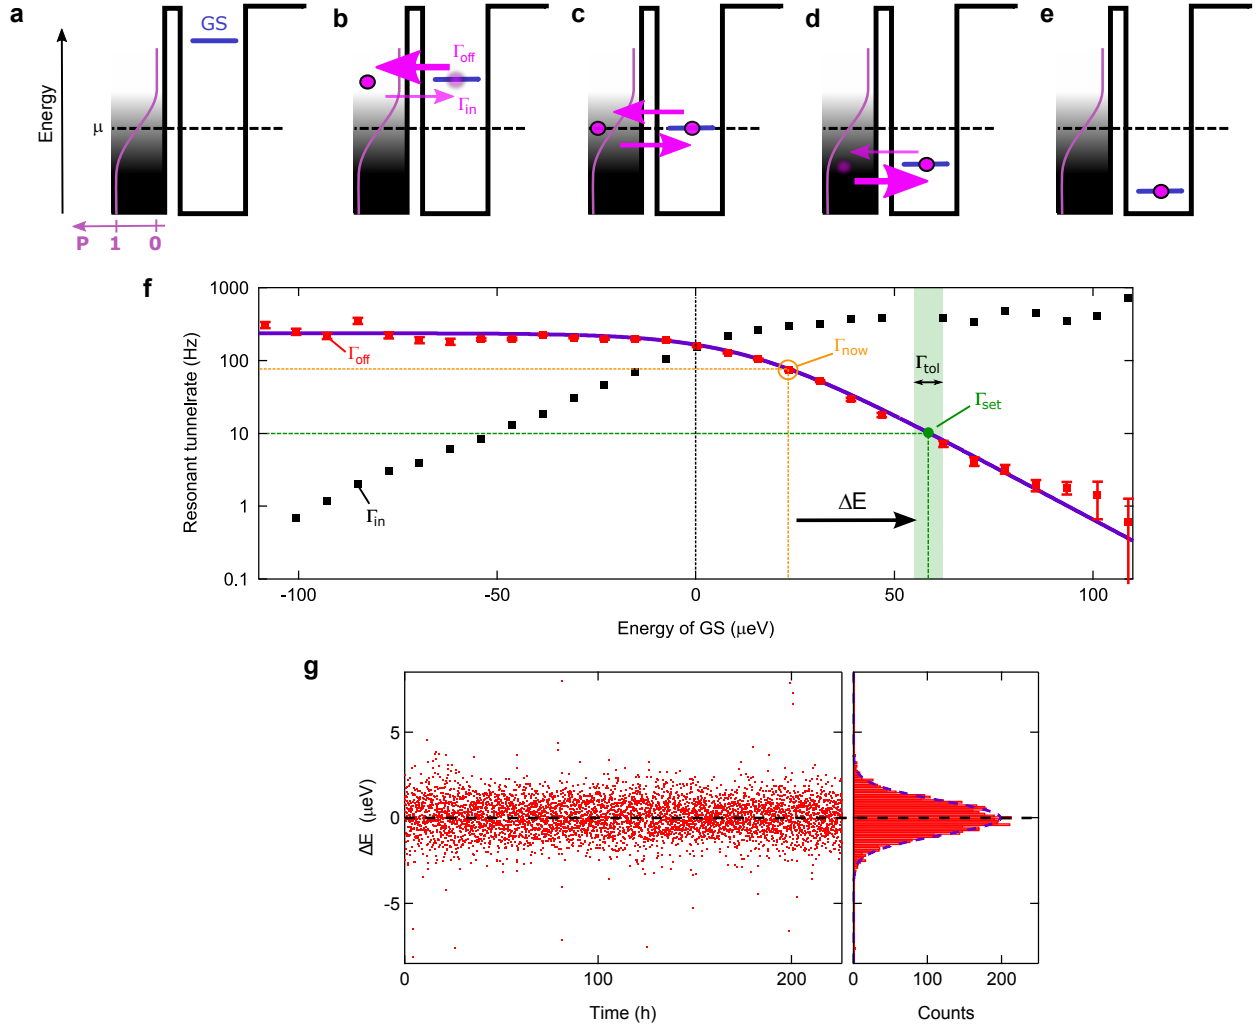

FIG. S3. **Level positioning algorithm (LPA).** **a-e** Schematics of tunnel rates (purple arrows) for different positions of the ground state with respect to  $\mu$ . The purple curve in the reservoir (left) depicts the probability of finding an electron in the reservoir as a function of energy. **f** Energy dependence of resonant tunnel rate out of the dot  $\Gamma_{off}$  (red square).  $\Gamma_{in}$  exhibits Fermi-Dirac statistics around the regime of resonant tunneling. The electron temperature is around 200 mK. The ground state of the dot drifts over time.  $\Gamma_{tol}$  of  $\Gamma_{set}$  is the tolerance interval, which, in practice, is usually set to be 10% of  $\Gamma_{set}$ , as shown by the green shaded region. For illustration an example for a correction is shown: if the measured tunnel off rate  $\Gamma_{now}$  is beyond the tolerance interval, the corresponding plunger gate is corrected by  $\Delta E$  to reset the initial position the ground state. This process is repeated in a closed-loop until  $\Gamma_{set}$  is restored. **g** The stability of the quantum dot is represented by the correction  $\Delta E$  for one spin relaxation measurement whereas the LPA is performed about every three minutes. A histogram of  $\Delta E$  is shown on the right side of the panel. The data exhibits a Gaussian distribution centered at 0 with standard deviation of  $1.4 \mu\text{eV}$ . It demonstrates that the dot is very stable.

the spin excited state is much larger than for the spin ground state which is needed for the spin-to-charge conversion (see Supplementary Section S3).

In Fig. S3g, a series of 5000 corrections ( $\Delta E$ ) are shown for a single spin relaxation measurement at 0.7 T over

a continuous measuring time of almost 10 days. For this measurement, the spin ground state is maintained at  $\Gamma_{off} = 10\text{ Hz}$ . We record resonant tunneling (Fig. S2) for 14s and extract the rates  $\Gamma_{in,off}$ . Note that  $\Gamma_{off}$  is equivalent to the background rate  $\Gamma_b$  described in the spin-to-charge conversion in Supplementary Section S3. The LPA allows measurements relying on precise alignment of the dot energy levels for an extended period of time, which is crucial to acquire enough data to provide statistics for extractions of long spin relaxation times.

Next, we turn to corrections of the sensor quantum dot. The best sensitivity is achieved when the sensor is positioned on the steepest point of a Coulomb peak (see Fig. S4a). To preserve this operation point, a feedback is regularly carried out to compensate for sensor drifts. Before the sensor feedback was carried out, the main dot is slightly detuned from  $\mu$  to avoid resonant tunneling and a stable  $I_{SQD}$  is read. Drift results in changes of the sensor dot energy spectrum indicated in Fig. S4a. This leads to a change of  $I_{SQD}$  and more severely to a reduction in sensitivity ( $dI_{SQD}/dV_{SP}$ ). By applying corrections to the sensor plunger  $SP$  (Fig. S4b) in a closed loop, the original sensor operation point is restored. These corrections are calculated with the flank of the Coulomb peak being linearly approximated in  $V_{SP}$ . In Fig. S4b, the evolution of applied voltage on  $SP$ ,  $V_{SP}$ , is shown for the same spin relaxation measurement discussed in Fig. S3. In contrast to Fig. S3g, only a few and solely positive corrections were carried out. This unidirectional behavior is often seen but its origin is not clear.

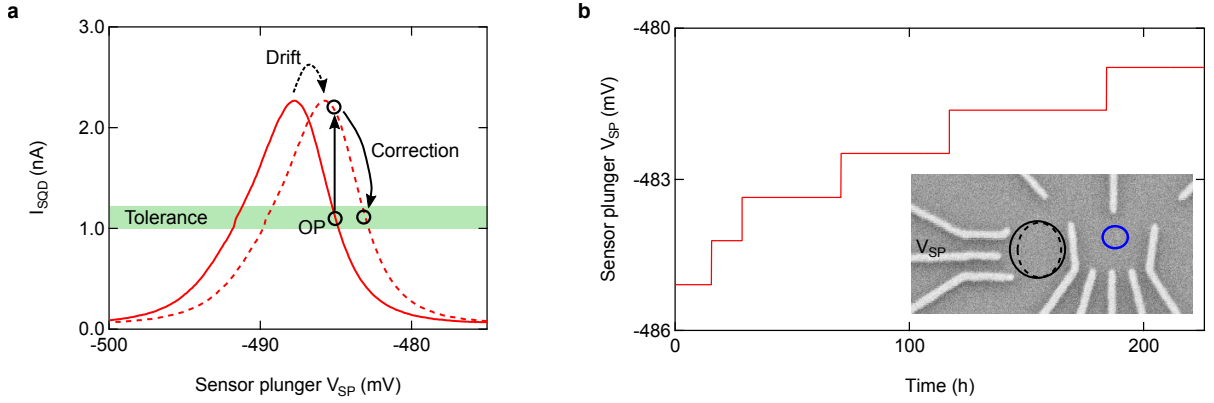

FIG. S4. **Sensor feedback.** **a**  $I_{SQD}$  of a sensor Coulomb peak (red solid curve) with the sensor operation point (OP, black circle). With time, the Coulomb peak shifts in energy and hence in plunger voltage  $V_{SP}$  (red dashed curve). This changes the sensor signal as well as the sensitivity indicated by the vertical arrow. To restore the original operation point,  $V_{SP}$  is adjusted until  $I_{SQD}$  is once more within a tolerance. **b** The effective voltage on  $SP$  for a long measurement showing corrections to compensate drift. The carried out corrections are of similar magnitude because the feedback is only applied as soon as  $I_{SQD}$  is out of the tolerance. The inset schematically shows the sensor dot becoming more confined (dashed circle) due to the drift.

### S3. SPIN RELAXATION MEASUREMENT SCHEME

In this section we present the rate equations for the three step pulse measurement scheme necessary to extract the spin relaxation rate  $W$ . This section gives a brief summary of the rate equations solved in Ref. 1.

#### 3a. Ionization

Both spin-up and spin-down states are pulsed well above  $\mu$  for several ms. If the dot is occupied, the electron will

tunnel off immediately so that the dot will be empty or ionized. We intentionally choose the duration and the ground state energy detuning such that an ionization probability  $> 99\%$  is achieved.

### 3b. Charge and Relax

In the charge and relax pulse step, both spin states are pulsed below  $\mu$  (see Fig. S5a). During the waiting time  $t_w$ , only four pathways are possible: (1) the dot stays empty; (2) an electron tunnels into the spin ground state; (3) an electron tunnels into and stays in the spin excited state; (4) an electron tunnels into the spin excited state and relaxes into the spin ground state. There are other suppressed paths like exchange with the reservoir after loading. Such alternative events are found not to influence the statistics and therefore are neglected. In simplified terms, the measurement scheme relies on counting electrons taking path (3) and tunneling out the excited state during the spin-to-charge conversion because they are not yet relaxed. Under the assumption that the dot is ionized in the beginning of the charge and relax step (see Fig. S5a), the rate equation for the probability for the dot being empty is

$$\dot{P}_{empty}(t) = -\Gamma_{in}P_{empty} \rightarrow P_{empty}(t) = e^{-\Gamma_{in}t}. \quad (1)$$

$$\Gamma_{in} = (\Gamma_e + \Gamma_g) \quad (2)$$

Note that  $P_{empty}(t) = 1 - P_L(t)$  with  $P_L$  the loading probability during the charge and relax step. Although the individual coupling of the spin excited and ground states to the reservoir,  $\Gamma_e$  and  $\Gamma_g$ , is unknown<sup>5-7</sup>, the total coupling  $\Gamma_{in}$  can be obtained by two different methods. Fig. S5b shows  $P_{empty}(t_w)$ , the probability distribution of the dot being empty when entering the read-out stage (3c) after waiting time  $t_w$  in the charge and relax stage. This probability is fitted to an exponential function to find  $\Gamma_{in}$ . In the second method,  $\Gamma_{in}$  is obtained by a fit to the histogram of  $t_{on}$ 's, the times for an electron to tunnel into the empty dot (Fig. S5c). The drawback of this method is that in addition to the readout the sensor must also be sensitive during the charge and relax stage to detect  $t_{on}$ . We therefore apply a compensation pulse to sensor plunger gate SP (see inset of Fig. S4b) to retain sensitivity. This method also allows to obtain  $\Gamma_{in}$  for each waiting time  $t_w$  individually. As shown in Fig. S5d,  $\Gamma_{in}$  is independent of  $t_w$  as expected.

Without considering the contribution due to the thermal excitation from the spin ground state, the rate equation of the probability for an electron being in the spin excited state is  $\dot{P}_e = \Gamma_e P_{empty} - W P_e$ . By solving this equation, we find the probability distribution

$$P_e(t) = \frac{\Gamma_e}{\Gamma_{in}} \cdot \frac{\Gamma_{in}}{\Gamma_{in} - W} \cdot (e^{-Wt} - e^{-\Gamma_{in}t}). \quad (3)$$

Note that  $\frac{\Gamma_e}{\Gamma_{in}}$ , which is not known, is only a scaling factor.

### 3c. Read out

When entering the read-out (RO) stage, the probability of the electron still being in the spin excited state after the charge and relax stage is  $P_e(t_w)$ . In the read-out stage, an electron can leave the spin excited state by either tunneling off the dot with a rate  $\Gamma_{off,e}^{RO}$  or by relaxing into the spin ground state with spin relaxation rate  $W$ . Thus, the rate equation for an electron tunneling out of the spin excited state is  $\dot{P}_e^{RO} = -\Gamma_{off,e}^{RO} P_e^{RO} - W P_e^{RO}$ , which leads to

$$P_e^{RO}(t) = P_e(t_w) \cdot e^{-(\Gamma_{off,e}^{RO} + W)t}. \quad (4)$$

For the spin ground state, either an electron in the spin excited state can relax with rate  $W$  or an electron can tunnel into the reservoir with background rate  $\Gamma_b$ . The rate equation is  $\dot{P}_g^{RO} = -\Gamma_b P_g^{RO} + W P_e^{RO}$ , whereas the spin excited

state is involved due to spin relaxation. The solution for this equation is

$$P_g^{RO}(t) = P_g(t_w)e^{-\Gamma_b t} + P_e(t_w) \cdot \frac{W}{\Gamma_{off,e}^{RO} + W - \Gamma_b} (e^{-\Gamma_b t} - e^{-(\Gamma_{off,e}^{RO} + W)t}), \quad (5)$$

where  $P_g(t_w) = 1 - P_e(t_w) - P_{empty}(t_w)$  is the probability for an electron to be in the spin ground state when entering the read-out configuration.  $P_g^{RO}(t)$  and  $P_e^{RO}(t)$  are not directly observable in the experiment. But we can detect the timing of tunnel events out of the quantum dot during the readout stage. The probability for an electron tunneling off at time  $t_{off}$  in the readout stage is  $P_{off}^{RO} = \Gamma_{off,e}^{RO} P_e^{RO}(t_{off}) + \Gamma_b P_g^{RO}(t_{off})$  which is equivalent to

$$P_{off}^{RO} = \eta \cdot P_e(t_w) (\Gamma_{off,e}^{RO} + W) e^{-(\Gamma_{off,e}^{RO} + W)t_{off}} + \left( P_g(t_w) + \frac{W}{\Gamma_{off,e}^{RO} + W - \Gamma_b} P_e(t_w) \right) \Gamma_b e^{-\Gamma_b t_{off}} \quad (6)$$

with  $\eta = \left( 1 - \frac{W\Gamma_b}{\Gamma_{off,e}^{RO}(\Gamma_{off,e}^{RO} + W - \Gamma_b)} \right) \frac{\Gamma_{off,e}^{RO}}{\Gamma_{off,e}^{RO} + W}$ , the fraction of electrons in the spin excited state which tunnel out before they relax into the spin ground state. For low fields,  $\Gamma_{off,e}^{RO} \gg W, \Gamma_b$  such that  $\eta \approx 1$  while at high fields  $W \sim \Gamma_{off,e}^{RO}$  and  $\eta$  is reduced to  $\Gamma_{off,e}^{RO}/(\Gamma_{off,e}^{RO} + W)$ . Note that for the measurements presented in Fig. 2 of the main text,  $\eta \approx 1$ , and thus has not been involved in the discussion for better readability.

### 3d. Extraction of W

Fig. S5e shows exemplary histograms of  $t_{off}$  for three waiting times  $t_w$  in the charge and relax stage. The counts out of the dot depend on the loading probability  $P_L(t_w)$  and the probability to relax into the spin ground state during  $t_w$ ,  $W$ . In first panel of Fig. S5e,  $t_w$  is short compared to  $1/\Gamma_{in} \sim 1kHz$  and the dot is mostly empty when entering the read-out stage. For the next panel,  $t_w > 1/\Gamma_{in}$  so that  $P_L$  is increased. But  $t_w < 1/W$  and there is an increased number of electrons in the spin excited state which have not yet relaxed when entering the read out stage. For the third panel,  $P_L \sim 1$  but also  $t_w > 1/W$  such that almost all electrons have relaxed into the spin ground state when entering the read-out stage. The total rate out of the excited state  $R = \Gamma_{off,e}^{RO} + W$  is independent of  $t_w$ , as shown in Fig. S5f. This allows us to extract  $\eta P_e$  by fitting Eq. (6) to our  $t_{off}$  histograms for  $t_w$ 's.  $\Gamma_b$  is set and fixed by the LPA as mentioned above. For low fields where  $\Gamma_{off,e}^{RO} \sim \Gamma_b$  we also explicitly fit out  $\Gamma_b$  giving excellent agreement with the values chosen for the LPA.

$\eta P_e$  is then plotted as a function of  $t_w$ . The spin relaxation rate  $W$  can be explicitly found out by fitting  $\eta P_e(t_w)$  to Eq. (3). As mentioned above,  $\Gamma_{in}$  is independently obtained from histograms of  $t_{on}$  or  $P_{empty}(t_w)$ . Note that  $\eta$  is only a scaling factor for Eq. (3) and does not affect our ability to extract  $W$ . Fig. S5g shows  $\eta P_e(t_w)$  for selected applied magnetic fields with the respective fits. For the first three panels  $W < \Gamma_{in}$  and the exponential increase in  $\eta P_e(t_w)$  is represented by  $\Gamma_{in}$  while the decay is characterized by  $W$ . For the last panel,  $W > \Gamma_{in}$  and the exponential increase is actually given by  $W$  and the loading rate  $\Gamma_{in}$  is seen in the decay.

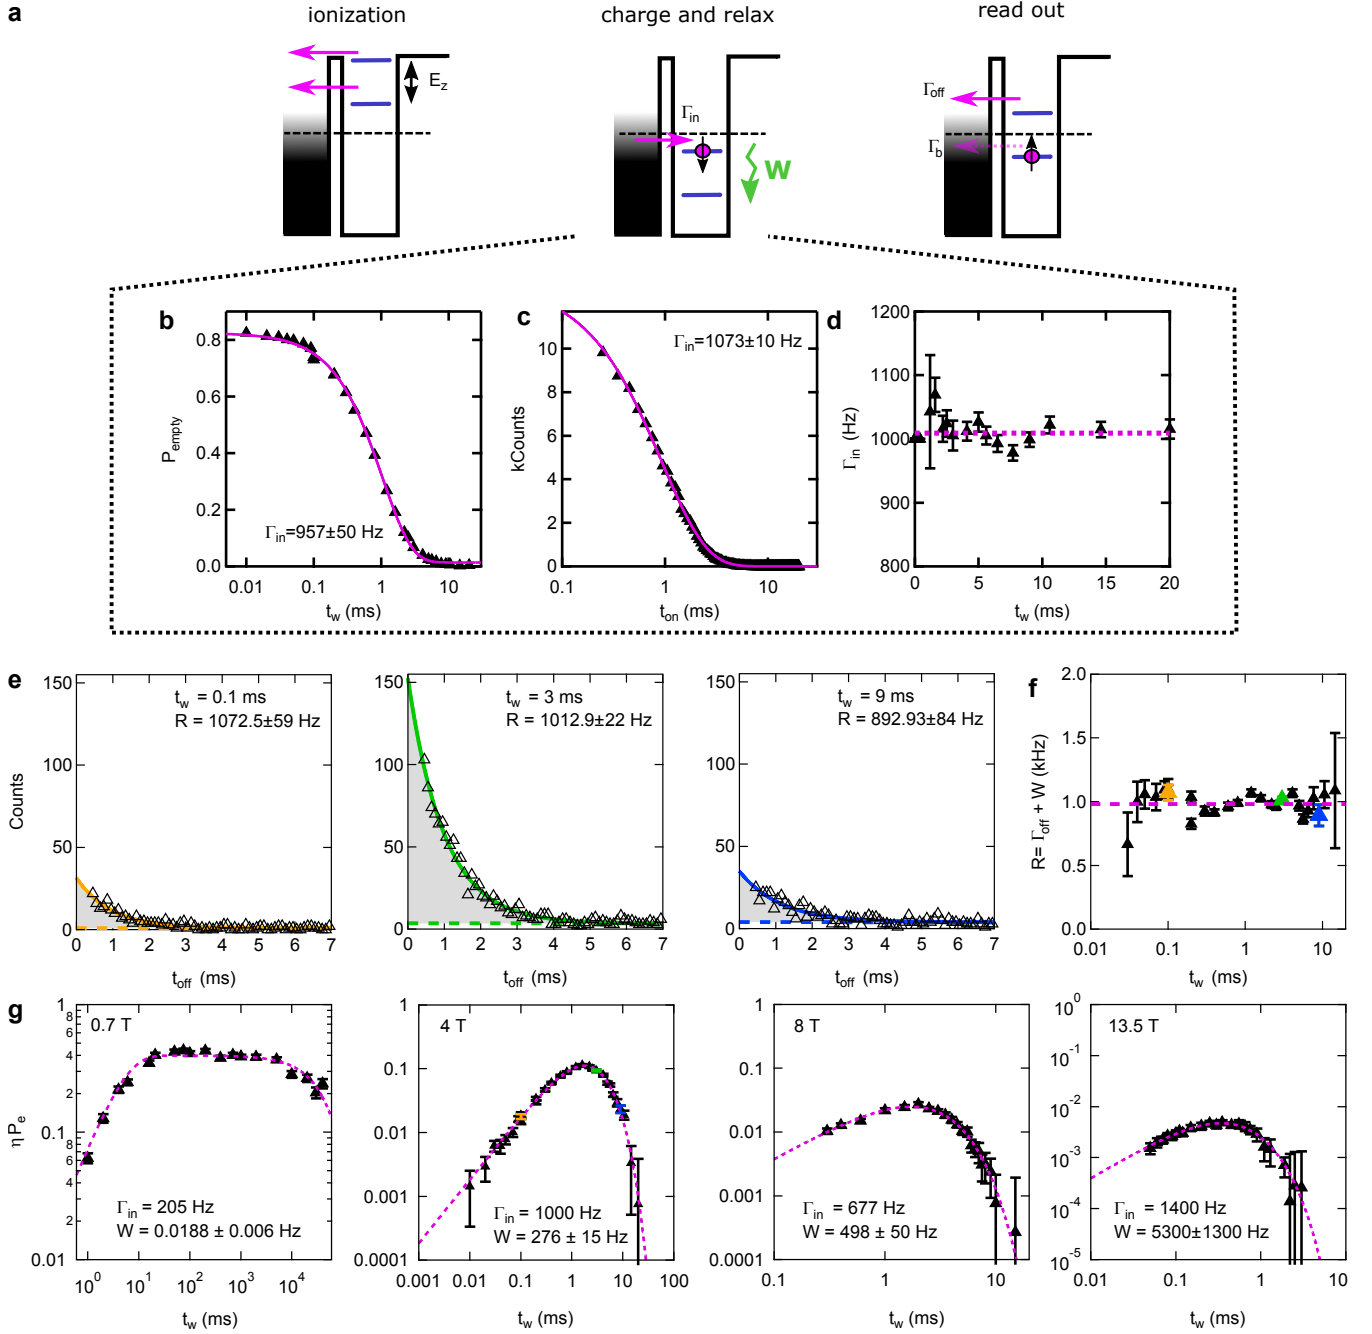

FIG. S5.  **$T_1$  measurement scheme.** **a** Schematics of the three-step pulse sequence used for the  $T_1$  measurement for Zeeman energy  $E_z = g\mu_B B$  and spin relaxation rate  $W$ . Methods to extract  $\Gamma_{in}$  by fitting ionization probability  $P_{empty}$  for different waiting times  $t_w$  (**b**) or by fitting the histogram of  $t_{on}$  for all data (**c**). **d** shows  $\Gamma_{in}$  at various waiting time  $t_w$  using the second extraction method. It shows that  $\Gamma_{in}$  is independent of  $t_w$ . **e** Histograms of tunnel off times  $t_{off}$  in the read-out stage for three different waiting times  $t_w$  exhibit a double exponential distribution with rates  $R = \Gamma_{off,e}^{RO} + W$  (solid line) and  $\Gamma_b$  (dashed) as described in the text. **f**  $R$  as a function of  $t_w$ . Colored datapoints correspond to colors adopted in **e**. **g**  $P_e$  for different  $t_w$  with fits to Eq. (3) as described in the text for four different fields.  $W$  can be then extracted accordingly.

#### S4. DEFINITIONS AND NOTATIONS FOR THE ELECTRON, NUCLEAR SPINS, AND PHONONS

We describe the quantum dot and the spin relaxation by the following model. The total electronic Hamiltonian is

$$H = T + V + H_Z + H_{SOI} + H_{HF}, \quad (7)$$

the components of which we now discuss. To this end, we define the coordinate system along the crystallographic directions by defining unit vectors  $\mathbf{x} \equiv [100]$ ,  $\mathbf{y} \equiv [010]$ , and  $\mathbf{z} \equiv [001]$  and the corresponding coordinates  $x$ ,  $y$ , and  $z$ . The heterostructure is grown along  $\mathbf{z}$ , and the wavefunction corresponding to the lowest 2DEG subband is  $\psi_0(z)$ . In the  $xy$ -plane, the electronic states are defined by the kinetic energy with the electron effective mass  $m$ , the anisotropy tensor  $\mathcal{M}$ , and a bi-quadratic confinement potential,

$$T + V = \frac{1}{2m} \mathbf{p} \cdot \mathcal{M} \cdot \mathbf{p} + \frac{\hbar^2}{2m} \left( \frac{(\mathbf{r} \cdot \mathbf{n}_1)^2}{l_1^4} + \frac{(\mathbf{r} \cdot \mathbf{n}_2)^2}{l_2^4} \right). \quad (8)$$

The tensor  $\mathcal{M}$  reflects the orbital effects of strong in-plane magnetic fields. It is diagonal in coordinate system with the first axis along the in-plane component of the magnetic field and the second perpendicular to it. In these coordinates  $\mathcal{M}^{-1} = \text{diag}(1, 1 + \Phi^2)$ , so that the mass along the in-plane field is unchanged, and perpendicular to it is enhanced. The enhancement grows with  $\Phi$ , the flux penetrating the 2DEG due to the field (see below). The confinement soft and hard potential axes,  $\mathbf{n}_1$  and  $\mathbf{n}_2$ , respectively, are slightly rotated, by angle  $\delta \approx 6^\circ$ , with respect to the device axes  $[110]$ , and  $[1\bar{1}0]$ . The confinement lengths  $l_1$  and  $l_2$  are related to the excitation energies by

$$E_1 = \hbar^2 / m l_1^2, \quad (9)$$

and an analogous equation for index 2.

The electron is subject to spin-dependent interactions. These comprise, first, the Zeeman term,

$$H_Z = \mu_F \boldsymbol{\sigma} \cdot \mathbf{B}, \quad (10)$$

where  $(\sigma_x, \sigma_y, \sigma_z) = \boldsymbol{\sigma}$  is the vector of sigma matrices,  $\mathbf{B} = B(\cos \xi \cos \phi, \cos \xi \sin \phi, \sin \xi)$  is the magnetic field, and  $\mu_F = (g/2)\mu_B$  is the reduced electron magnetic moment, with the g-factor  $g$ , and the Bohr magneton  $\mu_B$ . The associated Zeeman energy is  $\epsilon_z = g\mu_B B = 2\mu_F B$ . Second, the spin-orbit interactions. We split them to the linear Rashba and Dresselhaus terms,

$$H_{SOI}^{(1)} = \alpha (\sigma_y p_x - \sigma_x p_y) + \beta (-\sigma_x p_x + \sigma_y p_y), \quad (11)$$

and the cubic Dresselhaus term,

$$H_{SOI}^{(3)} = \frac{\gamma_c}{\hbar^3} (\sigma_x p_x p_y^2 - \sigma_y p_y p_x^2). \quad (12)$$

The linear interactions strengths are parameterized by a spin-orbit length  $l_{so}$ , and angle  $\vartheta$  by writing  $\alpha = (\hbar/2ml_{so}) \cos \vartheta$ , and  $\beta = (\hbar/2ml_{so}) \sin \vartheta$ . The linear spin-orbit terms can be recast, by a unitary transformation of the Hamiltonian, into the effective interaction<sup>8</sup>,

$$H_{SOI}^{\text{eff}} = \mu_F (\mathbf{n}_{so} \times \mathbf{B}) \cdot \boldsymbol{\sigma}, \quad (13)$$

which will be convenient below. The dimensionless spin-orbit vector

$$\mathbf{n}_{so}(\mathbf{r}) = \frac{x}{l_{so}} [\sin \vartheta, -\cos \vartheta, 0] + \frac{y}{l_{so}} [\cos \vartheta, -\sin \vartheta, 0], \quad (14)$$

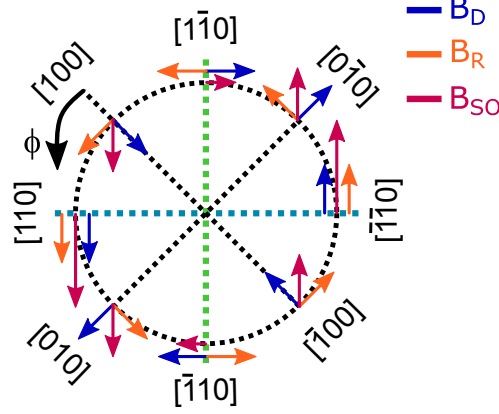

FIG. S6. **Angular spin orbit interaction.** The total SOI field  $B_{SOI} = B_R + B_D$  (red) along various crystal axes from the interplay of the Rashba  $B_R$  (orange) and linear Dresselhaus  $B_D$  (dark blue) SOI components. The interplay of  $B_R$  and  $B_D$  leads to an anisotropic  $B_{SO}$ . A maximal  $B_{SO} \sim |\alpha + \beta|$  is expected along  $[110]$  and minimal  $B_{SO} \sim |\alpha - \beta|$  along  $[1\bar{1}0]$ .  $\phi$  is defined as the angle with respect to  $[100]$ .

which we write using the dot coordinates as

$$\mathbf{n}_{\text{so}}(\mathbf{r}) = \mathbf{n}_{\text{so}}^{(1)}(\mathbf{n}_1 \cdot \mathbf{r}) + \mathbf{n}_{\text{so}}^{(2)}(\mathbf{n}_2 \cdot \mathbf{r}), \quad (15)$$

by defining the following vectors

$$\mathbf{n}_{\text{so}}^{(1)} = \frac{1}{l_{\text{so}}} [\sin(\delta + \vartheta), -\cos(\delta - \vartheta), 0], \quad (16a)$$

$$\mathbf{n}_{\text{so}}^{(2)} = \frac{1}{l_{\text{so}}} [\cos(\delta + \vartheta), \sin(\delta - \vartheta), 0]. \quad (16b)$$

For later convenience the following expressions are noted,

$$|\mathbf{n}_{\text{so}}^{(1)} \times \mu_F \mathbf{B}|^2 = \left( \frac{\mu_F B}{l_{\text{so}}} \right)^2 \left[ \cos^2 \xi \cdot (\cos \phi \cos(\delta - \vartheta) + \sin \phi \sin(\delta + \vartheta))^2 + \sin^2 \xi \cdot (1 + \sin 2\delta \sin 2\vartheta) \right], \quad (17)$$

$$|\mathbf{n}_{\text{so}}^{(2)} \times \mu_F \mathbf{B}|^2 = \left( \frac{\mu_F B}{l_{\text{so}}} \right)^2 \left[ \cos^2 \xi \cdot (\cos \phi \sin(\delta - \vartheta) - \sin \phi \cos(\delta + \vartheta))^2 + \sin^2 \xi \cdot (1 - \sin 2\delta \sin 2\vartheta) \right].$$

These expressions are anisotropic, what is rooted in the anisotropy of the spin-orbit interactions, Eq. (11), illustrated in Fig. S6. Third, the Fermi's contact interaction,

$$H_{HF} = Av_0 \sum_n \delta(z - z_n) \delta(\mathbf{r} - \mathbf{r}_n) \boldsymbol{\sigma} \cdot \mathbf{I}_n, \quad (18)$$

where  $n$  labels the nuclei with spin  $\mathbf{I}_n$  and position  $\mathbf{R}_n \equiv (\mathbf{r}_n, z_n)$ , and similarly  $\mathbf{R} = (\mathbf{r}, z)$  is the three dimensional electron position operator. Further,  $A$  is a material constant, and  $v_0 = a_0^3/8$  is the volume per atom, with  $a_0$  the lattice constant. To evaluate the matrix elements  $H_{HF}$ , one has to consider also the extension of the electronic state along the  $\mathbf{z}$  axis. We define the length scale  $l_h$  by<sup>9</sup>

$$l_h^{-1} = \int dz |\psi(z)|^4, \quad (19)$$

which therefore depends on the 2DEG width along the growth direction. The flux due to the in-plane field is also related to the 2DEG width, by

$$\Phi = \frac{e}{h} \lambda_z^2 B \cos \xi, \quad (20)$$

through another effective length  $\lambda_z$ . Both  $l_h$  and  $\lambda_z$  are of the order of the nominal width of the 2DEG,  $l_z$ , with the precise relation dependent on the heterostructure confinement profile, what is analyzed in Ref. 10.

The electron-phonon interaction is described by

$$H_{ph} = \sum_{\lambda\kappa} \left( b_{\lambda\kappa} + b_{\lambda-\kappa}^\dagger \right) H_{ph}^{\lambda\kappa}, \quad (21)$$

where  $\lambda \in \{l, t_1, t_2\}$  is the acoustic phonon branch index, with  $l$  the longitudinal and  $t_1, t_2$  the two transversal branches of acoustic phonons,  $\kappa$  is the three dimensional phonon wavevector, and the coupling

$$H_{ph}^{\lambda\kappa} = \sum_{\eta} \sqrt{\frac{\hbar\kappa}{2\rho V c_\lambda}} \sigma_\eta M_{\lambda\kappa}^\eta e^{i\kappa \cdot \mathbf{R}}. \quad (22)$$

For later notational convenience the index  $\eta \in \{df, pz\}$  labels here the electron-phonon interactions, deformation and piezoelectric. Further,  $\rho$  is the material density,  $V$  is the crystal volume,  $c_\lambda$  is the sound velocity,  $M_{\lambda\kappa}^{df} = \delta_{\lambda l}$  with the latter being the Kronecker delta symbol,  $\sigma_{df} = \sigma_e$  is the deformation potential,  $\sigma_{pz} = -ie h_{14}/\kappa$ , with  $h_{14}$  being the piezoelectric constant, and

$$M_{\lambda\kappa}^{pz} = \frac{2}{\kappa^2} (\kappa_x \kappa_y e_\lambda^z + \kappa_z \kappa_x e_\lambda^y + \kappa_y \kappa_z e_\lambda^x), \quad (23)$$

is a dimensionless factor defined by the components of  $\mathbf{e}_\lambda$ , the three mutually perpendicular polarization vectors of unit length.

## S5. THE SPIN RELAXATION RATE

The relaxation rate between an initial electronic state  $i$  and the final state  $f$ , with the corresponding energies  $E_i$ ,  $E_f$ , corresponding to a single phonon emission, is given by the Fermi's Golden rule

$$\Gamma = \frac{2\pi}{\hbar} \sum_{\lambda\kappa} |\langle f | H_{ph}^{\lambda\kappa} | i \rangle|^2 \delta(E_{if} - \hbar c_\lambda \kappa) [n(E_{if}) + 1], \quad (24)$$

where we assumed  $E_{if} = E_i - E_f > 0$ , and  $n$  is the phonon thermal occupation factor

$$n(\epsilon) = \frac{1}{\exp(\epsilon/k_B T) - 1}, \quad (25)$$

with  $k_B$  the Boltzmann constant and  $T$  the temperature.

For the spin relaxation, the initial state is  $|i\rangle = |\Psi_{0\downarrow}\rangle$ , the orbital ground state with spin down, the final state is  $|f\rangle = |\Psi_{0\uparrow}\rangle$ , the orbital ground state with spin up, and the transition energy equals to the Zeeman energy,  $E_{if} = \epsilon_z$ . In the continuum limit for phonons,  $\sum_{\kappa} \rightarrow [V/(2\pi)^3] \int d\kappa$ , we get Eq. (24) in the following form

$$\Gamma = [n(\epsilon_z) + 1] \sum_{\eta\lambda} \int d\kappa \frac{\kappa}{8\pi^2 \rho c_\lambda} |\sigma_\eta|^2 |M_{\lambda\kappa}^\eta|^2 |\tau(\kappa)|^2 \delta(\epsilon_z - \hbar c_\lambda \kappa), \quad (26)$$

where we introduced

$$\tau(\boldsymbol{\kappa}) = \langle \Psi_{0\downarrow} | e^{i\boldsymbol{\kappa} \cdot \mathbf{R}} | \Psi_{0\uparrow} \rangle, \quad (27)$$

as the matrix element of the electron-phonon interaction between the initial and final state. Even though our numerics implements the evaluation of these formulas exactly, to substantiate the discussion in the main text introduction, we also provide analytical results. To this end, we adopt some approximations, most importantly the dipole approximation, expanding the exponential in Eq. (27) to the lowest order. The quantity  $|\tau|^2$  is then given by the dipole matrix element between the lowest spin opposite quantum dot states and is bilinear in the components of vector  $\boldsymbol{\kappa}$  (see Supplementary Section S7). To proceed with such an expression, we define the following average

$$\langle f(\boldsymbol{\kappa}) \rangle = \int d\boldsymbol{\kappa} |M_{\lambda\boldsymbol{\kappa}}^\eta|^2 f(\boldsymbol{\kappa}) \delta(\epsilon_z - \hbar c_\lambda \kappa), \quad (28)$$

as the integral over phonons wavevectors with the weights from Eq. (26). The crystal symmetry then gives the following result

$$\langle (\boldsymbol{\kappa} \cdot \mathbf{n})(\boldsymbol{\kappa} \cdot \mathbf{m}) \rangle = C_\lambda^\eta \frac{\kappa_\lambda^4}{\hbar c_\lambda} (\mathbf{n} \cdot \mathbf{m}), \quad (29)$$

for  $\mathbf{n}$  and  $\mathbf{m}$  being in-plane unit vectors,  $\kappa_\lambda = \epsilon_z / \hbar c_\lambda$ , and the numerical constants being  $C_l^{df} = 2\pi/3$ ,  $C_l^{pz} = 8\pi/35$ , and  $C_{t_1}^{pz} = C_{t_2}^{pz} = 2/3 \times C_l^{pz}$ . We now write the rate as

$$\Gamma = \gamma \langle d^2 \rangle, \quad (30)$$

splitting it to the phonon part and the (averaged) dipole moment between the spin opposite states. The first is

$$\gamma = [n(\epsilon_z) + 1] \sum_{\eta\lambda} C_\lambda^\eta \frac{\kappa_\lambda^5}{8\pi^2 \hbar \rho c_\lambda^2} |\sigma_\eta|^2 = \frac{n(\epsilon_z) + 1}{15\pi \hbar \rho} \left( \frac{5}{4} \frac{\sigma_e^2}{\hbar^5 c_l^7} \epsilon_z^5 + \frac{(eh_{14})^2}{\hbar^3 c^5} \epsilon_z^3 \right), \quad (31)$$

where we defined a weighted phonon velocity

$$\frac{1}{\bar{c}^5} = \left( \frac{3}{7} \frac{1}{c_l^5} + \frac{4}{7} \frac{1}{c^5} \right). \quad (32)$$

The second, derived in Supplementary Section S7, is

$$|d_{SOI}|^2 \approx |\mu_F \mathbf{B} \times \mathbf{n}_{\text{so}}^{(1)}|^2 l_1^4 \frac{E_1^2}{(E_1^2 - \epsilon_z^2)^2} + |\mu_F \mathbf{B} \times \mathbf{n}_{\text{so}}^{(2)}|^2 l_2^4 \frac{E_2^2}{(E_2^2 - \epsilon_z^2)^2}, \quad (33a)$$

$$|d_{HF}|^2 \approx \frac{2I(I+1)}{3} \frac{A^2}{N} \left( l_1^2 \frac{E_1^2}{(E_1^2 - \epsilon_z^2)^2} + l_2^2 \frac{E_2^2}{(E_2^2 - \epsilon_z^2)^2} \right). \quad (33b)$$

Equations (31) and (33) make the power dependence on the magnetic field explicit for any combination of the phonon interaction, with  $\gamma^{df} \propto B^5$  and  $\gamma^{pz} \propto B^3$  and the spin-dependent electron interaction, with  $|d_{SOI}|^2 \propto B^2$ , and  $|d_{HF}|^2 \propto B^0$  (up to the small magnetic field orbital effects; see below). The expressions for the relaxation rates given in the Methods, Eq. (1) and (2), can be obtained by restricting to the dominant piezoelectric phonons in Eq. (31), neglecting the Zeeman term with respect to the orbital energies, and using Eq. (9), and for the spin-orbit interaction case also Eq. (17).

## S6. ANISOTROPY OF THE HYPERFINE RELAXATION RATE

The strong anisotropy of the relaxation induced by the spin-orbit interactions played a major role in our experiment and allowed to distinguish it from the hyperfine effects. Indeed, compared to the explicitly anisotropic Eq. (33a), the expression in Eq. (33b) stays unchanged, as long as the dot shape is fixed. Neglecting the orbital effects of the magnetic field, this is indeed the case. In this section we estimate the small anisotropy induced by going beyond this approximation (of a purely in-plane field, and a 2DEG with zero width). We first consider the orbital effects of a purely in-plane field, and then an out-of-plane field. For both of these it is useful to consider a change of the mass in the kinetic term of a linear harmonic oscillator,  $m \rightarrow m^*$ . With the Hamiltonian written in the form of Eq. (8),

$$\frac{p^2}{2m} + \frac{\hbar^2}{2m} \frac{r^2}{l^4} \rightarrow \frac{p^2}{2m^*} + \frac{\hbar^2}{2m} \frac{r^2}{l^4} \equiv \frac{p^2}{2m^*} + \frac{\hbar^2}{2m^*} \frac{r^2}{l^{*4}}, \quad (34)$$

Upon such a change the oscillator energy and dipole elements rescale to

$$E^* = E \left( \frac{m}{m^*} \right)^{1/2}, \text{ and } l^* = l \left( \frac{m}{m^*} \right)^{1/4}. \quad (35)$$

the latter following from  $E^* = \hbar/m^*l^{*2}$ , the standard relation for the LHO energy. The in-plane field orbital effects will therefore lead to such changes along the axis perpendicular to the magnetic field. If the dot is anisotropic, this will lead to anisotropic change of the dipole moment  $|d_{HF}|^2$ . We quantify the magnitude of such anisotropy by the ratio of the difference and sum, of the dipole moment extrema (as a function of the magnetic field direction), which are achieved with the magnetic field along the potential axes,

$$\Delta_{|d|^2}^{in} \equiv \frac{|d(\mathbf{B} \parallel \mathbf{n}_1)|^2 - |d(\mathbf{B} \parallel \mathbf{n}_2)|^2}{|d(\mathbf{B} \parallel \mathbf{n}_1)|^2 + |d(\mathbf{B} \parallel \mathbf{n}_2)|^2} = \frac{1 - (1 + \Phi^2)^{3/2} \frac{E_1^{-3} - E_2^{-3}}{E_1^{-3} + E_2^{-3}}}{1 + (1 + \Phi^2)^{3/2} \frac{E_1^{-3} + E_2^{-3}}{E_1^{-3} - E_2^{-3}}}. \quad (36)$$

The left hand equality sign is a definition, and the right hand side was obtained by neglecting the Zeeman energy in Eq. (33b), and using that the in-plane field renormalizes the mass according to  $m^*/m = 1 + \Phi^2$ , with the flux given in Eq. (20). The expression in Eq. (36) is plotted for our parameters in Fig. S7.

We now turn to the case of a magnetic field with an out-of-plane magnetic component,  $B \sin \xi \neq 0$ . We will consider an isotropic quantum dot, for simplicity, and define the anisotropy of the rate by comparing its value for a purely in-plane field, and a value for a finite out-of-plane component. With these two values, we define  $\Delta$  for this case analogously to Eq. (36). The orbital effects of an out-of-plane field are described by a renormalization of the confinement length, and splitting the excited states energies according to their orbital moment  $\mu$ . These two effects are for the two excited lowest states,  $\mu = \pm 1$ , given by

$$l^{*-4} = l^{-4} + \left( \frac{eB \sin \xi}{2\hbar} \right)^2, \text{ and } E^* = \frac{\hbar^2}{ml^{*2}} \pm \frac{\hbar e}{2m} B \sin \xi. \quad (37)$$

Calculating  $\Delta$  becomes a straightforward algebra, using the previous equation, and Eq. (33b), and we plot the result in Fig. S7. We note that for the case of a slightly asymmetric dot, the energy effect is quenched as long as  $(\hbar e/2m)B_z \ll |E_1 - E_2|$ , which is the case in our experiment. Keeping only the orbital squeezing effect (the renormalization of the confinement length), we then get

$$\Delta_{|d|^2}^{out} \equiv \frac{|d(\xi)|^2 - |d(\xi = 0)|^2}{|d(\xi)|^2 + |d(\xi = 0)|^2} \approx 3 \frac{e^2 B^2}{8\hbar^2} \sin^2 \xi. \quad (38)$$

Looking at the figure, we conclude that the expected anisotropies of the hyperfine relaxation rates due to the orbital effects of the magnetic field are indeed very small, and the hyperfine induced relaxation is therefore expected to be isotropic within the experimental resolution.

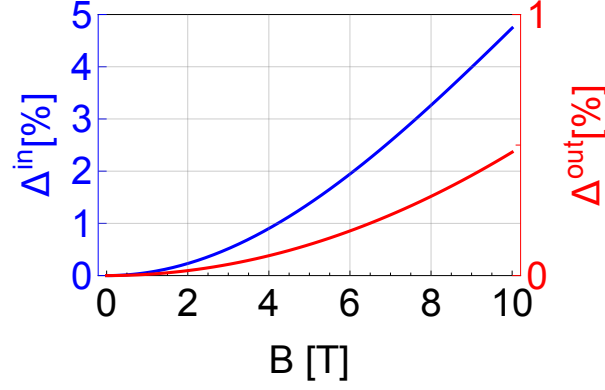

FIG. S7. **Anisotropy of the hyperfine induced relaxation rate.** The blue curve shows  $\Delta^{in}$ , Eq. (36), the in-plane the anisotropy of the relaxation rate. It equals the ratio of the maximal deviation of the rate from its average, and the average, upon varying the magnetic field within the 2DEG plane. The red curve shows  $\Delta^{out}$ , Eq. (38), the out-of-plane anisotropy of the rate (the full expression and its approximation are indistinguishable on the figure resolution). It shows, again on relative scale, the change of the rate upon misaligning the field out of the 2DEG plane. We adopted the parameters of the dot, and for the second quantity we set  $\xi = 1.3^\circ$ , the maximal misalignment angle found in Fig. S1b).

## S7. DIPOLE MATRIX ELEMENTS BETWEEN THE SPIN OPPOSITE STATES

We now derive Eq. (33), considering the spin-dependent effects (other than the Zeeman energy) in the Hamiltonian Eq. (7) perturbatively. To this end, we define the unperturbed Hamiltonian  $H_0 = T + V + H_Z$  and consider the effects of the remaining terms,  $H' = H_{SOI} + H_{HF}$  in the basis of the unperturbed eigenstates, denoted  $|\Phi\rangle$ , while the exact eigenstates are denoted by  $|\Psi\rangle$ . Both are labelled by the orbital and spin index of the electronic wavefunction,  $j = 0, 1, \dots$ , and  $\sigma = \uparrow, \downarrow$ , respectively, and the many-particle state of the nuclear spins in the quantum dot, denoted as a multi-index  $\mu$ .

With this notation, we calculate the matrix element in Eq. (27) in the lowest order perturbation in  $H'$ . Expanding the indexes by the one corresponding to the nuclear spins, the initial state is

$$|\Psi_{0\bar{\sigma}\mu}\rangle \approx |\Phi_{0\bar{\sigma}\mu}\rangle + \sum_{j\sigma'\mu' \neq 0\bar{\sigma}\mu} \frac{\langle \Phi_{j\sigma'\mu'} | H' | \Phi_{0\bar{\sigma}\mu} \rangle}{E_{0\bar{\sigma}\mu} - E_{j\sigma'\mu'}} |\Phi_{j\sigma'\mu'}\rangle, \quad (39)$$

where the phonon emission (absorption) corresponds to  $\sigma = \uparrow (\downarrow)$ , while the final state is

$$|\Psi_{0\sigma\mu^*}\rangle \approx |\Phi_{0\sigma\mu^*}\rangle + \sum_{j\sigma'\mu' \neq 0\sigma\mu^*} \frac{\langle \Phi_{j\sigma'\mu'} | H' | \Phi_{0\sigma\mu^*} \rangle}{E_{0\sigma\mu^*} - E_{j\sigma'\mu'}} |\Phi_{j\sigma'\mu'}\rangle. \quad (40)$$

We assume that the unperturbed basis can be factorized

$$|\Phi_{j\sigma\mu}\rangle = |\Phi_j\rangle \otimes |\sigma\rangle \otimes |\mu\rangle, \quad (41)$$

so that the orbital part does not depend on the spin indexes, and that the electron-phonon interaction, the matrix element of which we are calculating, is diagonal in both spin indexes. This gives

$$\tau(\kappa) = \sum_j \langle \bar{\sigma}\mu | \frac{e^{i\kappa \cdot \mathbf{R}_{0j}} H'_{j0}}{E_{0j} + (E_{\sigma\bar{\sigma}} + E_{\mu^*\mu})} + \frac{e^{i\kappa \cdot \mathbf{R}_{j0}} H'_{0j}}{E_{0j} - (E_{\sigma\bar{\sigma}} + E_{\mu^*\mu})} | \sigma\mu^* \rangle, \quad (42)$$

where we have introduced the notation for orbital matrix elements as

$$O_{ij} = \langle \Phi_i | O | \Phi_j \rangle, \quad (43)$$

for energies as  $E_{ij} = E_i - E_j$ , and similarly for the spin indexes. Note also that the  $j = 0$  term cancels exactly from the sum in Eq. (42).

We now adopt the dipole approximation, by expanding the electron-phonon interaction to the lowest order

$$e^{i\boldsymbol{\kappa} \cdot \mathbf{R}} \approx 1 + i\boldsymbol{\kappa} \cdot \mathbf{R}, \quad (44)$$

which leads to

$$\tau(\boldsymbol{\kappa}) = i\boldsymbol{\kappa} \cdot \sum_{j \neq 0} \langle \bar{\sigma}\mu | \frac{\mathbf{R}_{0j}H'_{j0}}{E_{0j} + (E_{\sigma\bar{\sigma}} + E_{\mu^*\mu})} + \frac{\mathbf{R}_{j0}H'_{0j}}{E_{0j} - (E_{\sigma\bar{\sigma}} + E_{\mu^*\mu})} | \sigma\mu^* \rangle, \quad (45)$$

This leads to substantial simplification for a bi-harmonic quantum dot. Indeed, in such a case only the lowest two excited states have non-zero dipole matrix element with the ground state, which are mutually orthogonal (even if they are complex, which is, however, not considered here). In this case, the integration over the phonon wavevectors  $\boldsymbol{\kappa}$  makes the mixed terms in  $|\tau|^2$  zero, see Eq. (29). We therefore get

$$\langle |\tau(\boldsymbol{\kappa})|^2 \rangle = \langle |\boldsymbol{\kappa} \cdot \mathbf{d}_1|^2 \rangle + \langle |\boldsymbol{\kappa} \cdot \mathbf{d}_2|^2 \rangle, \quad (46)$$

where the dipole moments for the excited states are given by

$$\mathbf{d}_j = \langle \bar{\sigma}\mu | \frac{\mathbf{R}_{0j}H'_{j0}}{E_{0j} + (E_{\sigma\bar{\sigma}} + E_{\mu^*\mu})} + \frac{\mathbf{R}_{j0}H'_{0j}}{E_{0j} - (E_{\sigma\bar{\sigma}} + E_{\mu^*\mu})} | \sigma\mu^* \rangle. \quad (47)$$

Next we evaluate these dipole elements separately for the spin-orbit, and hyperfine interactions. We will also neglect the nuclear Zeeman energies  $E_{\mu^*\mu}$  as negligible compared to the electron Zeeman energy  $E_{\sigma\bar{\sigma}} = \bar{\sigma}\epsilon_z$ , and notice that we can put  $\mathbf{R}_{ij} = \mathbf{r}_{ij}$ , if all considered states are from the lowest 2DEG subband, what is the case here.

Let us take first the spin-orbit interactions. We take into account only the linear terms in their effective form,  $H' = H_{SOI}^{\text{eff}}$ , and neglect the cubic term, and ignore nuclear effects, by putting  $\mu^* = \mu$ . Since the effective spin-orbit interaction is also of the dipole operator form, we easily get

$$|\mathbf{d}_j|_{SOI}^2 = |\mathbf{r}_{0j}|^4 |\mathbf{n}_{so}^{(j)} \times \mu_F \mathbf{B}|^2 \frac{4E_{0j}^2}{(E_{0j}^2 - \epsilon_z^2)^2}. \quad (48)$$

Using here the results for the Fock-Darwin eigenfunctions,  $\mathbf{r}_{01} = (l_1/\sqrt{2})\mathbf{n}_1$ , and  $\mathbf{r}_{02} = (l_2/\sqrt{2})\mathbf{n}_2$ , and Eq.(46) gives Eq. (33a). The calculation for the hyperfine interaction proceeds analogously, and we get

$$|\mathbf{d}_j|_{HF}^2 = (Av_0)^2 \sum_{mn} \left( \frac{\mathbf{r}_{0j}\delta_{j0}^n}{E_{0j} + E_{\sigma\bar{\sigma}}} + \frac{\mathbf{r}_{j0}\delta_{0j}^n}{E_{0j} - E_{\sigma\bar{\sigma}}} \right) \cdot \left( \frac{\mathbf{r}_{j0}\delta_{0j}^m}{E_{0j} + E_{\sigma\bar{\sigma}}} + \frac{\mathbf{r}_{0j}\delta_{j0}^m}{E_{0j} - E_{\sigma\bar{\sigma}}} \right) \langle \bar{\sigma}\mu | \mathbf{I}_n \cdot \boldsymbol{\sigma} | \sigma\mu^* \rangle \langle \sigma\mu^* | \mathbf{I}_m \cdot \boldsymbol{\sigma} | \bar{\sigma}\mu \rangle, \quad (49)$$

where we denoted  $\delta_{ij}^n = [\delta(\mathbf{R} - \mathbf{R}_n)]_{ij}$ . The expression in Eq. (49) depends on the initial and final state of the nuclear subsystem. The experimentally relevant situation is that these two states are not restricted in any way, which corresponds to a rate being summed over all possible final states and averaged, with the proper statistical weights, over the possible initial states,

$$\overline{|\mathbf{d}|^2} = \sum_{\mu\nu} p(\mu) |\mathbf{d}(\mu, \nu)|^2. \quad (50)$$

A straightforward calculation for an unpolarized nuclear ensemble,  $p(\mu) = \text{const}$ , gives

$$\overline{\langle \sigma \mu | \mathbf{I}_m \cdot \boldsymbol{\sigma} | \bar{\sigma} \nu \rangle \langle \bar{\sigma} \nu | \mathbf{I}_n \cdot \boldsymbol{\sigma} | \sigma \mu \rangle} = \frac{2}{3} I(I+1) \delta_{nm}, \quad (51)$$

with  $\delta$  the Kronecker delta. Using this in Eq. (49) we get

$$|\mathbf{d}_j|^2_{HF} = A^2 \frac{2}{3} I(I+1) |\mathbf{r}_{0j}|^2 \frac{4E_{0j}^2}{(E_{0j}^2 - \epsilon_z^2)^2} v_0^2 \sum_m |\Phi_0(\mathbf{R}_m)|^2 |\Phi_j(\mathbf{R}_m)|^2. \quad (52)$$

As the linear density of the nuclear spins,  $2/a_0$ , is very high compared to the lengthscale of the electronic wavefunctions,  $l_1, l_2, l_z$ , the sum over nuclei can be well approximated by an integral,  $v_0 \sum_m \rightarrow \int d\mathbf{R}$ . Defining inverse volumes as the following wavefunction overlaps

$$V_{0j}^{-1} = \int d\mathbf{R} |\Phi_0(\mathbf{R})|^2 |\Phi_j(\mathbf{R})|^2, \quad (53)$$

the harmonic model gives  $V_{00} = 2\pi l_1 l_2 l_h$ , and  $V_{01} = V_{02} = 4\pi l_1 l_2 l_h$ . Putting  $N = V_{00}/v_0$  as the number of the nuclei "within" the quantum dot volume, leads to Eq. (33b) by using Eq. (52) in Eq. (46).

## S8. NUMERICAL IMPLEMENTATION

The spin relaxation rates are obtained inserting the numerically exact eigenstates into Eq. (24) and performing the integration over the phonon momenta numerically, by standard methods<sup>11</sup>. Whenever the Hamiltonian includes the hyperfine interaction, the given relaxation rate is an average of rates for 1000 configurations of static nuclear spins with random orientations (the approximation of unpolarized nuclei at infinite temperature). Specifically, the rate obtained at run  $i$  is written as  $\Gamma_i = \exp(\gamma_i)$ , and the average rate is defined as  $\Gamma_{\text{mean}} \equiv \exp(\bar{\gamma})$ , while the "error bar" given on such a value is defined by the maximal and minimal rates being  $\Gamma_{\text{max/min}} = \exp(\bar{\gamma} \pm \delta\gamma)$ , with  $\delta\gamma^2$  the dispersion of the exponents  $\gamma_i$ . This definition is chosen for convenience of resulting in a symmetric "error" interval on a logarithmic plot, so that the minimal rate stays non-zero, irrespective of the degree of the fluctuations among the individual rates. It should be taken only as a way to compare the degree of fluctuations among two values from numerics, rather than an assessment of fluctuations possibly observed in the experiment, since the latter depend in a non-trivial way on the relation between the measurement total time and the nuclear ensemble ergodic time<sup>12</sup>.

## S9. PARAMETERS AND FITTING OF THE SPIN-ORBIT CONSTANTS

In the evaluation of the rates according to the above described model, we use the parameters of GaAs,  $\rho = 5300 \text{ kg/m}^3$ ,  $c_l = 4784 \text{ m/s}$ ,  $c_t = 3350 \text{ m/s}$ ,  $\sigma_e = 7 \text{ eV}$ ,  $h_{14} = 1.4 \times 10^9 \text{ V/m}$ ,  $m = 0.067 m_e$ ,  $\gamma_c = 11 \text{ eV}\text{\AA}^3$ ,  $I = 3/2$ ,  $A = 45 \text{ }\mu\text{eV nm}$ ,  $a_0 = 5.65 \text{ }\text{\AA}$ . We also estimate the electron temperature  $T = 60 \text{ mK}$ , though the corresponding thermal factor in Eq. (25) is negligible even for highest magnetic fields, so that the temperature plays little role for the value of the spin relaxation (it can be set to zero in Eq. (24) leading to no visible changes). In addition to these parameters, we extract the excitation energies  $E_x = 2.3 \text{ meV}$  and  $E_y = 2.6 \text{ meV}$ , corresponding to  $l_x \approx 22 \text{ nm}$ , and  $l_y \approx 21 \text{ nm}$ , and the g-factor  $g = -0.36$ , from the spectral data such as those shown on Fig. 1c)-d) of the main text, and their spin-resolved analogues. As noted in the above and in the main text, to match the experimental relaxation rates quantitatively, one needs further details on the dot shape. As explained in detail in Ref. 10, we fit  $l_z = 6.5 \text{ nm}$ ,

and  $\delta = 5.6 \pm 1^\circ$ , which gives  $l_h/l_z = 2.4$ ,  $\lambda_z/l_z = 1.009$  upon assuming a triangular confinement potential along the heterostructure growth direction.

With all these values fixed, we fit the linear spin-orbit lengths by minimizing the following chi-square sum

$$\chi^2 = \sum_i \left( \ln \Gamma_{theory}^{(i)} - \ln \Gamma_{exp}^{(i)} \right)^2 w_i, \quad (54)$$

with respect to the fitting parameters  $l_{so}$  and  $\vartheta$ . In the sum the index  $i$  runs through the whole measured dataset of the relaxation rates  $\Gamma = 1/\mathbf{T}_1$  and we take the logarithm of the rate as they span a range of many orders of magnitude. The weights are chosen as  $w_i = \ln(1.05 + \delta\Gamma_{exp}^{(i)}/\Gamma_{exp}^{(i)})$ , with  $\delta\Gamma$  the error estimated when fitting the value of  $\Gamma$ , as explained in Fig. S5. However, we find that the extracted values of  $l_{so}$  and  $\vartheta$  are rather robust to many other choices (including ignoring the errors altogether). We find that the minimization converges into the following two local minima

$$l_{so} = 2.1(1) \mu\text{m}, \vartheta = 31(1)^\circ, \quad (55a)$$

$$l_{so} = 2.1(1) \mu\text{m}, \vartheta = 61(1)^\circ. \quad (55b)$$

where the values in the brackets give the typical error on the last given digit. These errors are estimated from the spread of the converged values upon running the minimization algorithm many times. The reason that we are not able to quantify these errors more precisely, is due to several uncertainties pertaining to the experimental as well as numerical inputs to the chi square sum. For example, the numerical value  $\Gamma_{theory}^{(i)}$  is a random variable, due to the randomness in the nuclear configuration. For the minimization, which is very computationally demanding, we are able to perform an average over typically only tens of random nuclear configurations for each  $i$ , which makes these statistical fluctuations quite large. For the same reasons, we are not able to quantify the likelihood ratio for the two local minima given in Eq. (55). However, using again multiple runs, we conclude that the difference between the two possibilities is, within our model, statistically significant, and the value  $\vartheta = 31^\circ$  fits the measured data better. Figure S8 illustrates the amount of data used to calculate  $\chi^2$  in the described minimization procedure.

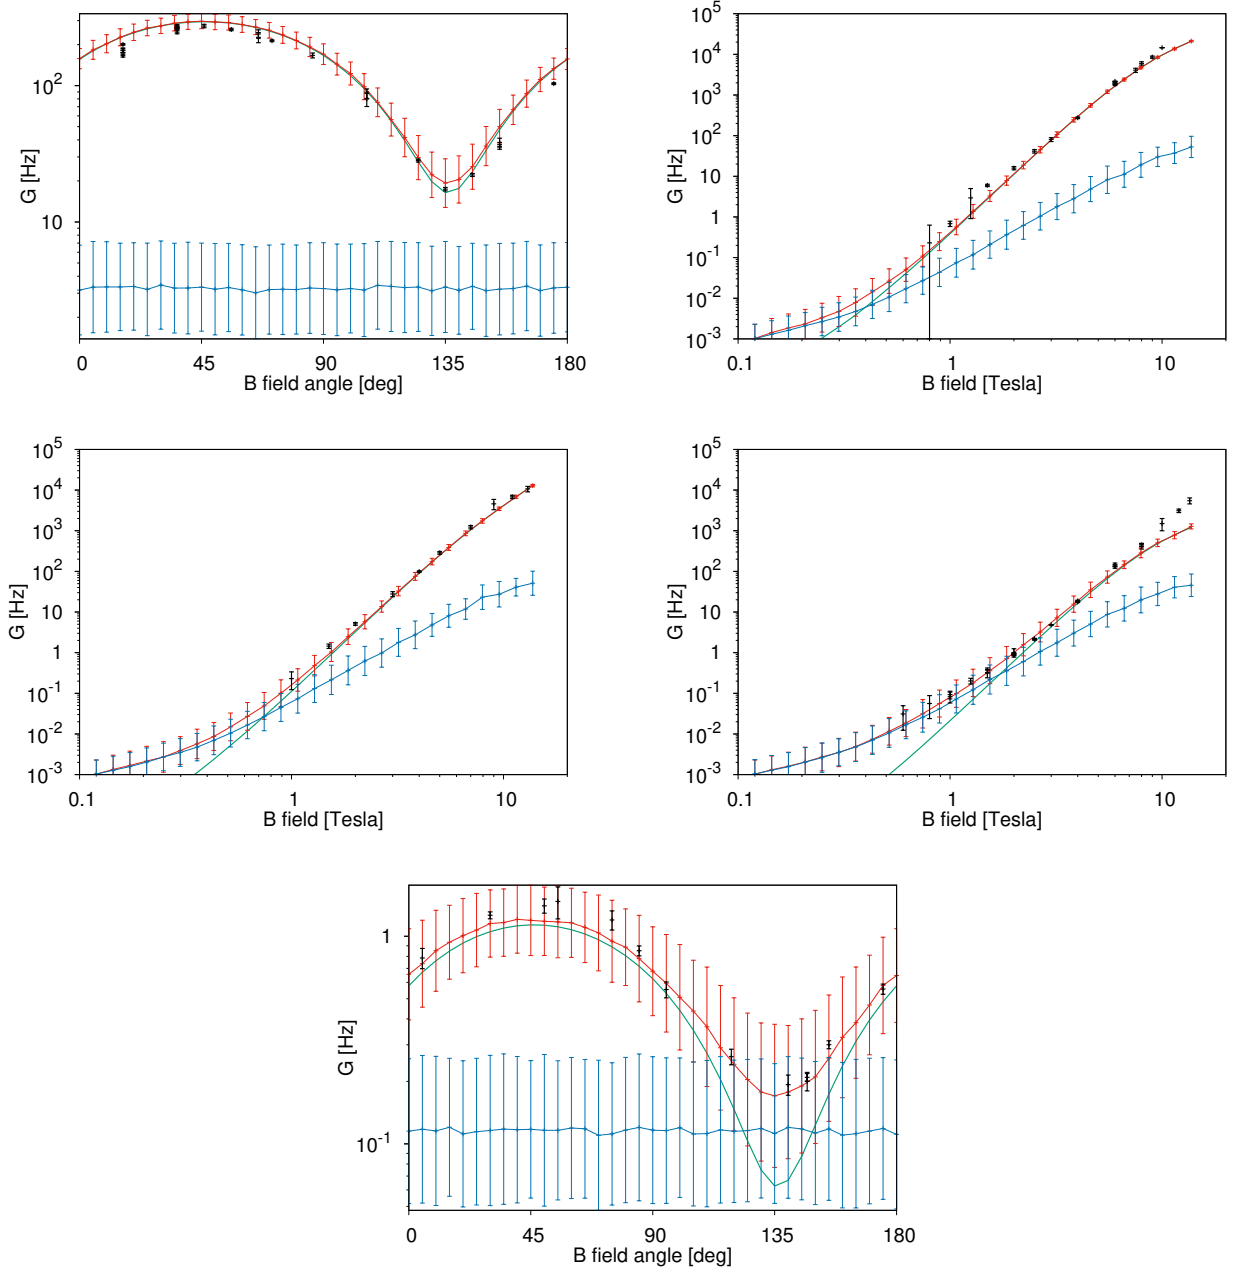

FIG. S8. **The total set of  $T_1$  data used to fit the spin-orbit parameters.** In all panels, we show the measured spin relaxation rates (black points with error bars) versus the theoretical values (lines) for the full model (red), the model excluding the hyperfine interactions (green) and the model excluding the spin-orbit effects (blue). The plotted values were obtained for  $\vartheta = 31.3^\circ$  and  $l_{so} = 2.08 \mu\text{m}$  and illustrate a single step in the minimization routine. Typically less than hundred steps are needed for convergence.

---

\* These authors contributed equally to this work

- <sup>1</sup> Amasha, S. *et al.* Measurements of the spin relaxation rate at low magnetic fields in a quantum dot. *arXiv*: 0607110 (2006). URL <http://arxiv.org/abs/cond-mat/0607110>.
- <sup>2</sup> Nazarov, Y. V. & Blanter, Y. M. *Quantum Transport* (Cambridge University Press, Cambridge, 2009).
- <sup>3</sup> Gustavsson, S. *et al.* Counting Statistics of Single Electron Transport in a Quantum Dot. *Phys. Rev. Lett.* **96**, 076605 (2006). URL <https://link.aps.org/doi/10.1103/PhysRevLett.96.076605>.
- <sup>4</sup> MacLean, K. *et al.* Energy-Dependent Tunneling in a Quantum Dot. *Phys. Rev. Lett.* **98**, 036802 (2007). URL <https://link.aps.org/doi/10.1103/PhysRevLett.98.036802>.
- <sup>5</sup> Amasha, S. *et al.* Spin-dependent tunneling of single electrons into an empty quantum dot. *Phys. Rev. B* **78**, 041306 (2008).
- <sup>6</sup> House, M. G. *et al.* Detection and Measurement of Spin-Dependent Dynamics in Random Telegraph Signals. *Phys. Rev. Lett.* **111**, 126803 (2013). URL <https://link.aps.org/doi/10.1103/PhysRevLett.111.126803>.
- <sup>7</sup> Yamagishi, M., Watase, N., Hashisaka, M., Muraki, K. & Fujisawa, T. Spin-dependent tunneling rates for electrostatically defined GaAs quantum dots. *Phys. Rev. B* **90**, 035306 (2014).
- <sup>8</sup> Baruffa, F., Stano, P. & Fabian, J. Theory of anisotropic exchange in laterally coupled quantum dots. *Phys. Rev. Lett.* **104**, 126401 (2010). URL <https://link.aps.org/doi/10.1103/PhysRevLett.104.126401>.
- <sup>9</sup> Merkulov, I. A., Efros, A. L. & Rosen, M. Electron spin relaxation by nuclei in semiconductor quantum dots. *Phys. Rev. B* **65**, 205309 (2002). URL <http://link.aps.org/doi/10.1103/PhysRevB.65.205309><https://link.aps.org/doi/10.1103/PhysRevB.65.205309>.
- <sup>10</sup> Stano, P. *et al.* Orbital effects of an in-plane field (2017). Preprint.
- <sup>11</sup> Press, W. H., Teukolsky, S. A., Vetterling, W. T. & Flannery, B. P. *Numerical Recipes 3rd Edition: The Art of Scientific Computing* (Cambridge University Press, New York, NY, USA, 2007), 3 edn.
- <sup>12</sup> Delbecq, M. R. *et al.* Quantum Dephasing in a Gated GaAs Triple Quantum Dot due to Nonergodic Noise. *Phys. Rev. Lett.* **116**, 046802 (2016). URL <https://link.aps.org/doi/10.1103/PhysRevLett.116.046802>.
